# Supplementary material for: Spatial and Statistical Modeling of Multi-Panel Millimeter Wave Self-Interference
Source: arXiv:2210.08093 source file (2023-03-04)
Supplement: Supplementary file 1 [file sec-appendix.tex]

\appendices

\section{Test}
